# Supplementary material for: Invariance-Aware Randomized Smoothing Certificates
Source: arXiv:2211.14207 source file (2023-01-03)
Supplement: Supplementary file 1 [file tight_backup.tex]

\subsection{Proof of Theorem 3}
Recall our main theorem for finding the worst-case classifier under invariance constraints.
\canonicalcert*
Further recall the definitions
\definitionequivalenceclasses*
and
\canonicalrepresentation*
and
\begin{equation*}
    \sH_\sT = \left\{h : \sR^{N \times D} \rightarrow \sY \mid
  \Pr_{\mZ \sim \mu_\mX} \left[h(\mZ) = y\right]
   \geq
  p_{\mX,y^*}
  \land \forall \mZ, \forall \mZ' \in \left[\mZ\right]_\sT : h(\mZ) = h(\mZ')
\right\}
\end{equation*}

We begin our proof of~\cref{theorem:canonical_cert} by proving the following lemmata:
\begin{lemma}\label{lemma:unique_representative}
    Let $\gamma$ be a canonical representation for invariance under $\sT$. Then, for all $\mZ \in \sR^{N \times D}$
    \begin{equation*}
        \mZ \neq \gamma(\mZ) \implies \nexists \mZ'\in \sR^{N \times D} : \gamma(\mZ') = \mZ.
    \end{equation*}
\end{lemma}
\begin{proof}
    Proof by contraposition.
    Assume there was some $\mZ'$ with $\gamma(\mZ') = \mZ$.
    \cref{eq:canonical_representation_1} would imply that $\mZ \in \left[\mZ'\right]_\sT$.
    \cref{eq:canonical_representation_2} would then imply that $\gamma(\mZ') = \gamma(\mZ)$.
    By the transitive property, we would have $\mZ = \gamma(\mZ') = \gamma(\mZ)$.
\end{proof}
The above lemma shows that if an input $\mZ$ is not the representative of its own equivalence class, then it cannot be the representative of any equivalence class.
\begin{lemma}\label{lemma:simplify_worstcase_set}
    Let $\gamma$ be a canonical representation for invariance under $\sT$.
    Then
    \begin{equation*}
        \forall \mZ, \forall \mZ' \in \left[\mZ\right]_\sT : h(\mZ) = h(\mZ') 
        \iff
        \forall \mZ: h(\mZ) = h(\gamma(\mZ)).
    \end{equation*}
\end{lemma}
\begin{proof}
    \item[$\Rightarrow$]
    Consider an arbitrary $\mZ \in \sR^{N \times D}$.
    Due to definition~\cref{eq:canonical_representation_1}, we know that $\gamma(\mZ) \in \left[\mZ\right]_\sT$.
    Therefore, $\forall \mZ' \in \left[\mZ\right]_\sT : h(\mZ) = h(\mZ')$ implies $h(\mZ) = h(\gamma(\mZ))$.
    \item[$\Leftarrow$]
    Consider an arbitrary pair of inputs $\mZ \in \sR^{N \times D}, \mZ' \in \left[\mZ\right]_\sT$.
    Due to~\cref{eq:canonical_representation_1}, we know  $\gamma(\mZ) \in \left[\mZ\right]_\sT$.
    Due to the definition of equivalence classes, we know that there must be some transformation $\tau \in \sT$ s.t.\ $\gamma(\mZ) = \tau(\mZ)$ and thus $h(\mZ) = h(\tau(\mZ)) = h(\gamma(\mZ))$.
    Due to~\cref{eq:canonical_representation_2}, we know that $\gamma(\mZ) = \gamma(\mZ')$ and
    thus $h(\gamma(\mZ)) = h(\gamma(\mZ'))$.
    We can again use~\cref{eq:canonical_representation_1} to show that there must be some transformation $\tau' \in \sT$ s.t.\ $\gamma(\mZ') = \tau'(\mZ')$ and thus $h(\gamma(\mZ')) =  h(\tau(\mZ')) = h(\mZ')$.
    By the transitive property, we have $h(\mZ) = h(\gamma(\mZ)) = h(\gamma(\mZ')) = h(\mZ')$.
\end{proof}

\cref{lemma:simplify_worstcase_set} allows us to restate $\sH_\sT$ as follows:
\begin{equation*}
    \sH_\sT = \left\{h : \sR^{N \times D} \rightarrow \sY \mid
  \Pr_{\mZ \sim \mu_\mX} \left[h(\mZ) = y\right]
   \geq
  p_{\mX,y^*}
  \land \forall \mZ : h(\mZ) = h(\gamma(\mZ))
\right\}.
\end{equation*}
Thus, the optimization problem $\min_{h \in \sH_\sT} \Pr_{\mZ \sim \mu_{\mX'}} \left[h(\mZ) = y^*\right]$ can be written as
\begin{align*}
    \min_{h : \sR^{N \times D} \rightarrow \sY} & \Pr_{\mZ \sim \mu_{\mX'}} \left[h(\mZ) = y^*\right]
    \\
    \text{ s.t. }& \Pr_{\mZ \sim \mu_{\mX}} \left[h(\mZ) = y^*\right] \geq p_{\mX, y^*}
    \land
     \forall \mZ : h(\mZ) = h(\gamma(\mZ)).
\end{align*}
Since we already know from the second constraint that any feasible solution must fulfill $h(\mZ) = h(\gamma(\mZ))$, we may as well substitute $h(\gamma(\mZ))$ for $h(\mZ)$  before solving the problem:
\begin{align}\label{eq:proof_canonical_cert_1}
    \begin{split}
    \min_{h : \sR^{N \times D} \rightarrow \sY} & \Pr_{\mZ \sim \mu_{\mX'}} \left[h(\gamma(\mZ)) = y^*\right]
    \\
    \text{ s.t. }& \Pr_{\mZ \sim \mu_{\mX}} \left[h(\gamma(\mZ)) = y^*\right] \geq p_{\mX, y^*}
    \land
     \forall \mZ : h(\mZ) = h(\gamma(\mZ)).
    \end{split}
\end{align}
For each $\mZ \in \sR^{N \times D}$, we can now distinguish two cases:
If $\mZ = \gamma(\mZ)$, then the constraint $h(\mZ) = h(\gamma(\mZ))$ is trivially fulfilled and can thus be dropped.
If $\mZ \neq \gamma(\mZ)$, then~\cref{lemma:unique_representative} shows that $h(\mZ)$ does not appear in the objective function or first constraint of~\cref{eq:proof_canonical_cert_1}, because there is no other $\mZ'$ with $\gamma(\mZ') = \mZ$.
We can thus ignore the constraint, solve the optimization problem
\begin{align*}
    \min_{h : \sR^{N \times D} \rightarrow \sY}  \Pr_{\mZ \sim \mu_{\mX'}} \left[h(\gamma(\mZ)) = y^*\right]
    \text{ s.t. } \Pr_{\mZ \sim \mu_{\mX}} \left[h(\gamma(\mZ)) = y^*\right] \geq p_{\mX, y^*}
\end{align*}
and then let $h(\mZ) \gets h(\gamma(\mZ))$ to obtain an optimal, feasible solution to~\cref{eq:proof_canonical_cert_1}.

\subsection{Proof of Theorem 4 (translation-invariance)}
\subsubsection{Canonical representation}
In the following, we first verify the correctness of our canonical representation for translation. We then derive the corresponding tight certificate.

\begin{restatable}{lemma}{canonicalrepresentationtranslation}\label{lemma:canonical_representation_translation}
    The function
        $\gamma(\mZ) = \mZ - \ones_N \mZ_{1,:}^T$
    is a canonical representation for translation-invariance.
\end{restatable}

\canonicalrepresentationtranslation*
\begin{proof}
    Based on the definition of canonical representations and translation-invariance, we need to show that 
    \begin{equation*}
        \forall \mZ \in \sR^{N \times D}: \gamma(\mZ) \in \left[\mZ\right]_\sT,
    \end{equation*}
    and
    \begin{equation*}
        \forall \mZ \in \sR^{N \times D}, \forall \mZ' \in \left[\mZ\right]_\sT : \gamma(\mZ) = \gamma(\mZ'),
    \end{equation*}
    $\left[\mZ\right]_\sT = \left\{\mZ + \ones_N \vc^T \mid \vc \in \sR^{N \times D}\right\}$.

    The function $\gamma$ performs a translation with $\vc = \mZ_{1,:}$, so the first criterion is fulfilled.
    
    Now, consider an arbitrary pair of matrices $\mZ, \mZ' \in \sR^{N \times D}$ with $\mZ' \in \left[\mZ\right]_T$, 
    i.e.~$\mZ' = \mZ + \ones_N  \vc^T$ for some $\vc$.
    We know that $\mZ'_{1,:} = \mZ_{1,:} + \vc$ and thus
    \begin{equation*}
        \gamma(\mZ') = \mZ' - \ones_N \mZ'_{1,:} = \left(\mZ + \ones_N \vc^T\right) - \ones_N \left(\mZ_{1,:} +\vc\right)^T
        = 
        \mZ - \ones_N \mZ_{1,:}^T
        = \gamma(\mZ),
    \end{equation*}
    meaning the second criterion is fulfilled as well.
\end{proof}





\subsubsection{Certificate}

To derive the robustness certificate for translation-invariance, we need the following lemmata:\todo{Betrag von determinante überall!}
%\normalchangeofvariables*
\begin{lemma}\label{lemma:inner_product_mean}
    Consider an arbitrary vector $\vx \in \sR^D$ and let $\overline{\vx} = \frac{1}{D}\sum_{d=1}^D \evx_d$ be its average.
    Then
    \begin{align*}
        \vx^T \left(\vx - \ones_D \overline{\vx}\right)
        = 
        \left(\vx - \ones_D \overline{\vx}\right)^T \left(\vx - \ones_D \overline{\vx}\right).
    \end{align*}
\end{lemma}
\begin{proof}
    We substract the left-hand side from the right-hand side
    \begin{align*}
        &\vx^T \left(\vx - \ones_D \overline{\vx}\right)
        = 
        \left(\vx - \ones_D \overline{\vx}\right)^T \left(\vx - \ones_D \overline{\vx}\right) \\
        \iff
        &
        0 = \left(- \ones_D \overline{\vx}\right)^T \left(\vx - \ones_D \overline{\vx}\right)\\
        \iff
        &
        0 = \sum_{d=1}^D \overline{x}^2 - \sum_{d=1}^D \evx_d \overline{x} \\
        \iff
        &
        0 = D \overline{x}^2 - D \overline{x}^2,
    \end{align*}
    where the last equality follows from the fact that $\sum_{d=1}^D \evx_d = D \overline{x}$.
\end{proof}

We can now turn to deriving our certificate.
Note that we mostly follow the procedure described in~\cref{section:certification_methodology}.
The only difference is that, rather than invoking the Neyman-Pearson lemma, we notice that the lower-dimensional optimization problem obtained from applying the canonical representation is equivalent to finding a tight certificate for a specific anisotropic Gaussian smoothing distribution.
Tight anisotropic Gaussian smoothing certificates have already been derived in prior work.
We can apply the known result to our specific mean and covariance matrix and then work through some additional linear algebra to derive our result.
\todo{ref}
\translationcert*
\begin{proof}
    First, we reformulate the canonical representation $\gamma$ from ~\cref{lemma:canonical_representation_translation} as $\gamma(\mZ) = \mK \mZ$ with $\mK = 
        \begin{bmatrix}
            0 & \zeros_{N-1}^T \\
            - \ones_{N-1} & \eye_{N-1}
        \end{bmatrix}$. The multiplication $\mK \mZ$ sets the first row of $\mZ$ to zero and subtracts the first row from all other rows, just like our originally defined $\gamma$.

    Applying~\cref{theorem:canonical_cert} with~\cref{lemma:canonical_representation_translation} shows that  the l.h.s.\ problem is equivalent to
    \begin{align*}
        \min_{h : \sR^{N \times D} \rightarrow \sY}   \Pr_{\mZ \sim \mu_{\mX'}} \left[h(\mK\mZ) = y^*\right]
    \text{ s.t. } \Pr_{\mZ \sim \mu_{\mX}} \left[h(\mK \mZ) = y^*\right] \geq p_{\mX, y^*}.
    \end{align*}
    
    We notice that the above optimization problem does not depend on the specific class predicted by $h$, but only on whether it is $y^*$ or $y$.
    To avoid clutter, we formulate the equivalent problem 
    \begin{align}\label{eq:proof_translation_1}
        \min_{h : \sR^{N \times D} \rightarrow \{0,1\}}   \mathbb{E}_{\mZ \sim \mu_{\mX'}} \left[h(\mK\mZ)\right]
    \text{ s.t. } \mathbb{E}_{\mZ \sim \mu_{\mX}} \left[h(\mK \mZ)\right] \geq p_{\mX, y^*},
    \end{align}
    where $h(\mZ) = 1$ indicates that $\mZ$ is classified as $y^*$.
    
    Recall that $\mu_\mX$ is an isotropic matrix normal distribution with variance $\sigma^2$. We thus have:
    \begin{align*}
         \mathbb{E}_{\mZ \sim \mu_{\mX}} \left[h(\mK \mZ)\right]
         &=
         \int_{\sR^{N \times D}}
         h(\mK \mZ) \prod_{d=1}^D \mathcal{N}\left(\mV_{:,d} \mid \mX_{:,d}, \sigma^2 \eye\right)
         \ d \mZ
    \end{align*}
    
    We can now use the substitution $\mA \mZ = \mV$ with
    $\mA =
    \begin{bmatrix}
        1 & \zeros_{N-1}^T\\
        -\ones_{N-1} & \eye_{N-1}
    \end{bmatrix}
    $,
    $\mA^{-1} = \begin{bmatrix}
        1 & \zeros_{N-1} \\
        \ones_{N-1} & \eye_N
    \end{bmatrix}$
    to simplify the integral.
    \begin{align*}
         \mathbb{E}_{\mZ \sim \mu_{\mX}} \left[h(\mK \mZ)\right]
         &=
         \int_{\sR^{N \times D}}
         h(\mK \mA^{-1} \mV) \mathrm{det}\left(\mA^{-1}\right)^D \prod_{d=1}^D \mathcal{N}\left(\mA^{-1} \mV_{:,D} \mid \mX_{:,d}, \sigma^2 \eye\right)
         \ d \mV
         \\
         &= 
         \int_{\sR^{N \times D}}
         h(\mK \mA^{-1} \mV) \prod_{d=1}^D \mathcal{N}\left(\mV_{:,d} \mid \mA\mX_{:,d}, \sigma^2 \mA \mA^T\right)
         \ d \mV
    \end{align*}
    The second equality follows from applying~\cref{lemma:normal_change_of_variables} $D$ times.
    Note that  
    $\mK \mA^{-1} = \begin{bmatrix}
        0 & \zeros_{N-1} \\
        \zeros_{N-1} & \eye_{N-1}
    \end{bmatrix}$.
    Since the first column is $0$ everywhere,  $h(\mK \mA^{-1} \mV)$ does not depend on the first row of $\mV$, meaning we can marginalize out $\mV_{1,1},\dots,\mV_{1,D}$.
    For multivariate normal distributions, this is equivalent to dropping the first row of the mean and the first row and column of the covariance matrix. In the following, we use $\mA_{2:} \in \sR^{(N-1)\times D}$ to denote the last $N-1$ rows of $\mA$.
    \begin{align*}
         &= 
         \int_{\sR^{N \times D}}
         h\left(
         \begin{bmatrix}
             \zeros_D\\
             \mV_{2:}
         \end{bmatrix}
         \right) \prod_{d=1}^D \mathcal{N}\left(\mV_{2:,d} \mid \mA_{2:}\mX_{:,d}, \sigma^2 \mA_{2:} \left(\mA_{2:}\right)^T\right)
         \ d \mV_{2:}.
         \\
    \end{align*}
    Let $\nu_\mX$ be this $((N-1) \times D)$-dimensional marginal distribution with density 
    $\nu_\mX(\mW) = 
    \prod_{d=1}^D \mathcal{N}\left(\mW_{:,d} \mid \mA_{2:}\mX_{:,d}, \sigma^2 \mA_{2:} \left(\mA_{2:}\right)^T\right).
    $
    We may then rewrite~\cref{eq:proof_translation_1} as
    \begin{align}\label{eq:proof_translation_2}
        \min_{h : \sR^{N \times D} \rightarrow \{0,1\}}   \mathbb{E}_{\mW \sim \nu_{\mX'}} \left[ h\left(
         \begin{bmatrix}
             \zeros_D\\
             \mW
         \end{bmatrix}
         \right)\right]
    \text{ s.t. } \mathbb{E}_{\mW \sim \nu_{\mX}} \left[ h\left(
         \begin{bmatrix}
             \zeros_D\\
             \mW
         \end{bmatrix}
         \right)\right] \geq p_{\mX, y^*},
    \end{align}
    Importantly, note that~\cref{eq:proof_translation_2} only depends on the function value of $h$ evaluated for matrices whose first row is zero. To use the family of variables analogy from~\cref{section:certification_methodology},~\cref{eq:proof_translation_2} only depends on a subset of variables indexed by $\sR^{(N-1) \times D}$. We may thus equivalently solve
    \begin{align}\label{eq:proof_translation_3}
        \min_{h : \sR^{(N-1) \times D} \rightarrow \{0,1\}}   \mathbb{E}_{\mW \sim \nu_{\mX'}} \left[ h\left(
             \mW
         \right)\right]
    \text{ s.t. } \mathbb{E}_{\mW \sim \nu_{\mX}} \left[ h\left(
             \mW
         \right)\right] \geq p_{\mX, y^*}.
    \end{align}
    At this point, we could apply the Neyman-Pearson lemma to exactly solve~\cref{eq:proof_translation_3}. However, this exact solution has already been derived in prior work.
    Note that the density function of $\nu_\mX$ is just the product of multiple multivariate normal density functions, which can be expressed as a single multivariate normal distribution with a block-diagonal covariance matrix.
    If $\mW \sim \nu_\mX$, then
    $\mathrm{vec}(\mW) \sim \mathcal{N}\left(\vm_\mX, \mSigma\right)$
    with $\vm \in \sR^{(N-1)D}$ and $\mSigma \in \sR^{(N-1)D\times(N-1)D}_+$,
    where
    \begin{align*}
        \vm_\mX &= \mathrm{vec}\left(\mA_{2:} \mX\right),\\
        \mSigma &= \begin{bmatrix}
        \mB & \zeros & \hdots & \zeros \\
        \zeros & \mB & \hdots & \zeros \\
        \vdots & \vdots & \ddots & \zeros \\
        \zeros & \zeros & \hdots & \mB
    \end{bmatrix}
    \end{align*}
    with $\mB = \sigma^2 \mA_{2:} \left(\mA_{2:}\right)^T$.
    We may thus restate~\cref{eq:proof_translation_3} as
    \begin{align}\label{eq:proof_translation_4}
        \min_{h' : \sR^{(N-1)D} \rightarrow \{0,1\}}   \mathbb{E}_{\vz \sim \mathcal{N}\left(\vm_{\mX'}, \mSigma\right)} \left[ h\left(
             \vz
         \right)\right]
    \text{ s.t. } \mathbb{E}_{\vz \sim \mathcal{N}\left(\vm_\mX, \mSigma\right)} \left[ h\left(
             \vz
         \right)\right] \geq p_{\mX, y^*}.
    \end{align}
    Note that any optimal solution to~\cref{eq:proof_translation_4} yields an optimal solution to~\cref{eq:proof_translation_3} with $h(\mZ) = h'(\mathrm{vec}(\mZ))$. To use the family of variables analogy: It is irrelevant whether we optimize over a family of variables indexed by $\sR^{(N-1) \times D}$ or one indexed by $\sR^{(N-1)D}$.
    
    \cref{eq:proof_translation_4} is the problem of finding a tight certificate for a classifier smoothed with anisotropic Gaussian noise. Its optimal value has been derived in \todo{cite} and is
    \begin{align*}
        \Phi\left(\Phi^{-1}\left(p_{\mX, y^*}\right) -
        \sqrt{
        \left(\vm_{\mX'} - \vm_{\mX}\right)^T \mSigma^{-1} \left(\vm_{\mX'} - \vm_{\mX}\right)
        }\right)
    \end{align*}
    We can conclude our proof by showing that
    \begin{align}
        \sqrt{
        \left(\vm_{\mX'} - \vm_{\mX}\right)^T \mSigma^{-1} \left(\vm_{\mX'} - \vm_{\mX}\right)
        }
        = \left\lvert\left\lvert \mDelta - \ones_N \overline{\mDelta}\right\rvert\right\rvert_2
    \end{align}
    First, we use the fact that the inverse of a block-diagonal matrix is also a block-diagonal matrix and insert the definitions of $\vm_{\mX'}$, $\vm_{\mX}$, $\mB$ to show that:
    \begin{align}
        &
        \left(\vm_{\mX'} - \vm_{\mX}\right)^T \mSigma^{-1} \left(\vm_{\mX'} - \vm_{\mX}\right)
        \\
        = &
        \left(\mathrm{vec}\left(\mA_{2:} \mX'\right) - \mathrm{vec}\left(\mA_{2:} \mX\right)\right)^T \mSigma^{-1} \left(\mathrm{vec}\left(\mA_{2:} \mX'\right) - \mathrm{vec}\left(\mA_{2:} \mX\right)\right)
\\
        = &
        \sum_{d=1}^D
        \left(\mA_{2:} \mX'_{:,d} - \mA_{2:} \mX_{:,d}\right)^T \mB^{-1} \left(\mA_{2:} \mX'_{:,d} - \mA_{2:} \mX_{:,d}\right)
    \\
        = &
        \sum_{d=1}^D
        \left(\mA_{2:} \mX'_{:,d} - \mA_{2:} \mX_{:,d}\right)^T
        \frac{1}{\sigma^2} \left(\mA_{2:} \left(\mA_{2:}\right)^T\right)^{-1}
        \left(\mA_{2:} \mX'_{:,d} - \mA_{2:} \mX_{:,d}\right)
 \\
        = &
        \frac{1}{\sigma}
        \sum_{d=1}^D
        \left(\mA_{2:} \mDelta_{:,d}\right)^T
         \left(\mA_{2:} \left(\mA_{2:}\right)^T\right)^{-1}
        \left(\mA_{2:}\mDelta_{:,d}\right),
         \\
        = &\label{eq:proof_translation_5}
        \frac{1}{\sigma}
        \sum_{d=1}^D
        \left(\mDelta_{:,d}\right)^T
         \left(\mA_{2:}\right)^T \left(\mA_{2:} \left(\mA_{2:}\right)^T\right)^{-1} \mA_{2:}
        \mDelta_{:,d},
    \end{align}
    where in the second to last last equation we have used that $\mX' = \mX + \mDelta$.
    
    Our next step is to compute $\left(\mA_{2:}\right)^T \left(\mA_{2:} \left(\mA_{2:}\right)^T\right)^{-1} \mA_{2:}$
    Recall that $\mA_{2:} \in \sR^{(N-1) \times D}$ and
    $\mA_{2:} =
    \begin{bmatrix}
        -\ones_{N-1} & \eye_{N-1}
    \end{bmatrix}
    $. Matrix multiplication shows that
    \begin{align*}
    \mA_{2:} \left(\mA_{2:}\right)^T = 
        \begin{bmatrix}
        -\ones_{N-1} & \eye_{N-1}
    \end{bmatrix}
    \begin{bmatrix}
        -\ones_{N-1} & \eye_{N-1}
    \end{bmatrix}^T
    = 
    \ones_{N-1,N-1} + \eye_{N-1}
    =
    \begin{bmatrix}
        2 & 1 & \hdots & 1 \\
        1 & 2 & \hdots & 1 \\
        \vdots & \vdots & \ddots & 1 \\
        1 & 1 & \hdots & 2
    \end{bmatrix}.
    \end{align*}
    The matrix is sufficiently simple to be inverted by inspection:
    \begin{equation*}
        \mA_{2:} \left(\mA_{2:}\right)^T
        = 
        \eye_{N-1} - \frac{1}{N} \ones_{N-1,N-1}
        =
        \begin{bmatrix}
        1 - \frac{1}{N} & - \frac{1}{N} & \hdots & - \frac{1}{N} \\
        - \frac{1}{N} & 1 -  \frac{1}{N} & \hdots & - \frac{1}{N} \\
        \vdots & \vdots & \ddots &   \frac{1}{N}\\
        - \frac{1}{N} & - \frac{1}{N} & \hdots & 1- \frac{1}{N}
    \end{bmatrix}.
    \end{equation*}
    Finally, matrix multiplication shows that
    \begin{align}\label{eq:proof_translation_6}
        \left(\mA_{2:}\right)^T \left(\mA_{2:} \left(\mA_{2:}\right)^T\right)^{-1} \mA_{2:}
        = 
        \eye_{N} - \frac{1}{N} \ones_{N,N}
        =
        \begin{bmatrix}
        1 - \frac{1}{N} & - \frac{1}{N} & \hdots & - \frac{1}{N} \\
        - \frac{1}{N} & 1 -  \frac{1}{N} & \hdots & - \frac{1}{N} \\
        \vdots & \vdots & \ddots &   \frac{1}{N}\\
        - \frac{1}{N} & - \frac{1}{N} & \hdots & 1- \frac{1}{N}
        \end{bmatrix}.
    \end{align}
    Note that~\cref{eq:proof_translation_6} transforms a vector by subtracting its average from all entries.
    Substituting into~\cref{eq:proof_translation_5} shows that
    \begin{align*}
        &\left(\vm_{\mX'} - \vm_{\mX}\right)^T \mSigma^{-1} \left(\vm_{\mX'} - \vm_{\mX}\right)\\
         =&
         \frac{1}{\sigma}
         \sum_{d=1}^D (\mDelta_{:,d})^T \left(\mDelta_{:,d} - \ones_D \overline{\mDelta_{:,d}}\right)\\
         =&
         \frac{1}{\sigma}
         \sum_{d=1}^D \left(\mDelta_{:,d} - \ones_D \overline{\mDelta_{:,d}}\right)^T \left(\mDelta_{:,d} - \ones_D \overline{\mDelta_{:,d}}\right)\\
         = &
         \frac{1}{\sigma}
         \sum_{n=1}^N\sum_{d=1}^D \left(\mDelta - \ones_N\overline{\mDelta}\right)_{n,d}^2,
    \end{align*}
    where $\overline{\mDelta} \in \sR^{1 \times D}$ is the column-wise average of $\mDelta$ and the second equality is due to~\cref{lemma:inner_product_mean}.
\end{proof}
Taking the square root and using the definition of the Frobenius norm yields our desired result:
\begin{equation*}
    \sqrt{
        \left(\vm_{\mX'} - \vm_{\mX}\right)^T \mSigma^{-1} \left(\vm_{\mX'} - \vm_{\mX}\right)
        }
        =
        \sqrt{\frac{1}{\sigma}
         \sum_{n=1}^N\sum_{d=1}^D \left(\mDelta - \ones_N\overline{\mDelta}\right)_{n,d}^2}
        = \left\lvert\left\lvert \mDelta - \ones_N \overline{\mDelta}\right\rvert\right\rvert_2.
\end{equation*}

\section{Proof of Theorem 5 (two-dimensional rotation-invariance)}
\subsection{Canonical representation}
Following the procedure described in~\cref{section:certification_methodology}, we first derive a canonical representation for invariance under translation in $2$D.
Recall that our group of transformations is $\sT = \left\{\mX \mapsto \mX \mR^T \mid \mR \in \mathit{SO}(2)\right\}$,
where $\mathit{SO}(2)$ is the special orthogonal group in two dimensions, i.e.\ the set of all rotation matrices.
Further recall the definition of canonical representations.
\canonicalrepresentation*

For our derivation, it is more convenient to work with polar coordinates. In the following, let
$\lambda : \sR^N \times \sR^N \rightarrow \sR^{N \times 2}$ with
$\lambda\left(\vr,\vtheta\right) =
\begin{bmatrix}
    \vr \odot \cos(\vtheta) & \vr \odot \sin(\vtheta)
\end{bmatrix}$
be the function that maps from polar coordinates into cartesian coordiantes. Here, $\odot$ is the elementwise product and $\cos$ and $\sin$ are applied element-wise.

First, we define a rotation operator for matrices:
\begin{definition}
    The matrix rotation operator is the function
    $\mathrm{rot} : \sR^{N \times 2} \times \sR \rightarrow \sR^{N \times 2 }$
    with
    \begin{align*}
    \mathrm{rot}(\mZ, a)
= \mZ \begin{bmatrix}
\cos(a) & - \sin(a) \\
\sin(a) & \cos(a)
\end{bmatrix}^T
\end{align*}
 that rotates all rows of matrix $\mZ$ by angle $a$.
\end{definition}

We use the matrix rotation operator to define our canonical representation,
which rotates all matrices $\mZ$ such that their first non-zero row is aligned with the first coordinate axis, i.e.~takes on value $0$ in the second column.
\begin{lemma}\label{lemma:canonical_representation_rotation_2d}
    The function $\gamma(\mZ) = \mathrm{rot}\left(\mZ, -\alpha(\mZ)\right)$
    with
    \begin{align*}
        \alpha(\mZ) = 
        \begin{cases}
            0 & \text{if } ||\mZ||_2 = 0 \\
            \mathrm{arctan2}\left(\mZ_{n^*,1},\mZ_{n^*,0}\right) & \text{else }
        \end{cases}
    \end{align*}
    where $n^* = \min\{n \mid ||\mZ_n||_2 > 0\}$ is the first non-zero row of matrix $\mZ$,
    is a canonical representation for rotation-invariance in $2$D.
\end{lemma}
\begin{proof}
    We can distinguish two cases.

    \textbf{Case 1.}
    All entries of $\mZ$ are $0$, i.e. $\mZ = \zeros_{N,2}$.
    In this case $||\mZ||_2 = 0$ and thus $\gamma(\mZ) = \mZ = \zeros_{N,2}$.
    The equivalence class of $\mZ$ is  $\left[\mZ\right]_\sT =
    \left\{\zeros_{N,2} \mR^T \mid \mR \in \mathit{SO}(2)\right\} = \{\zeros_{N,2}\}$.
    The criteria~\cref{eq:canonical_representation_1,eq:canonical_representation_2} for canonical representations are fulfilled.
    
    \textbf{Case 2.}
    The matrix $\mZ$ has non-zero entries.
    Let $\vr,\vtheta$ be a representation of $\mZ$ in polar coordinates, i.e. $\mZ = \lambda(\vr,\vtheta)$.
    Let $n^*$ be the index of the first non-zero row of $\mZ$.
    Recall that rotation in cartesian coordinates corresponds to translation of the polar coordiante angles and 
    thus $\gamma(\mZ) = \lambda(\vr,\vtheta - \ones_N \evtheta_{n^*})$.
    
    Criterion~\cref{eq:canonical_representation_1} is fulfilled, because by construction of $\gamma$ we have $\gamma(\mZ) = \mZ \sR^T$ for some $\sR^T$.
    
    Now, consider an arbitrary $\mZ' \in \left[\mZ\right]_\sT$.
    By definition of $\left[\mZ\right]_\sT$, there must be some $a \in \sR$ such that
    $\mZ' = \lambda\left(\vr,\vtheta + a\ones_N\right)$. Note that rotation does not affect the radii, i.e.\ $n^*$ is also the index of the first non-zero row of $\mZ'$.
    Thus
    \begin{align*}
        \gamma(\mZ') = \lambda\left(\vr,\vtheta + a\ones_N - \ones (\evtheta_{n^*} + a)\right) = 
        \lambda\left(\vr,\vtheta - \ones (\evtheta_{n^*})\right) = \gamma(\mZ),
    \end{align*}
    meaning criterion~\cref{eq:canonical_representation_2} is fulfilled as well.
\end{proof}

\subsection{Certificate}

\begin{lemma}
    Consider two multivariate normal distributions $\mathcal{N}(\mM_{:,1}, \mSigma), \mathcal{N}(\mM_{:,2}, \mSigma)$ with $\mM \in \sR^{N \times 2}$ that share the same symmetric covariance matrix $\mSigma^{-1} \in \sR^{N \times D}$.
    Further consider arbitrary $\vphi \in \sR^{N}$ and $\vr \in \sR^{N}$.
    Define $\vxi : \sR \times \sR^{N} \rightarrow \sR^{N}$ with $\vxi(\alpha, \vphi) =
                \vphi + \ones_{N} \alpha$
    Then
    \begin{align*}
        &\int\limits_{[0,2\pi]} \mathcal{N}
        \left(\vr \odot \cos\left(
            \vxi(\alpha,\vphi)
        \right) \mid \mM_{:,1}, \mSigma \right)
        \mathcal{N}\left(\vr \odot \sin\left(
            \vxi(\alpha,\vphi)
        \right) \mid \mM_{:,2}, \mSigma \right) \ d \alpha
        \\
        \propto & 
        \exp\left(
            -\frac{1}{2} \mathrm{vec}\left(\mM\right)^T
            \begin{bmatrix}
                \mSigma^{-1} & \zeros \\
                0 & \mSigma^{-1}
            \end{bmatrix}
            \mathrm{vec}\left(\mM\right)
        \right)
        \mathcal{I}_0\left(
        \left\lvert\left\lvert
         \vw
        \right\rvert\right\rvert_2
        \right)
        \\
        & \text{with } \vw = \begin{bmatrix}
            \mSigma^{-1} \mM_{:,1}  & \mSigma^{-1} \mM_{:,2} \\
            \mSigma^{-1} \mM_{:,2} & -\mSigma^{-1} \mM_{:,1} 
        \end{bmatrix}^T
        \begin{bmatrix}
            \lambda\left(\vr, \vphi\right)_{:,1} \\
            \lambda\left(\vr, \vphi\right)_{:,2}
        \end{bmatrix}.
    \end{align*}
    where $\cos$ and $\sin$ are applied element-wise, $\odot$ is the element-wise product and $\propto$ absorbs factors that are constant in $\mM$. Note that $\vw \in \sR^2$ and that $\mathcal{I}_0$ is the modified Bessel function of the first kind and order $0$.
\end{lemma}
\begin{proof}
    We begin by identifying terms that  that are constant in both $\mM$ and $\alpha$ and can thus be eliminated,
    as well as terms that are constant in $\alpha$ and can thus be moved outside the integral.
    We first eliminate the normalization constants:
    \begin{align*}
        & \mathcal{N}(
        \vr \odot \cos\left(
            \vxi(\alpha,\vphi)
        \right)
        \mid \mM_{:,1}, \mSigma) \mathcal{N}(
        \vr \odot \sin\left(
            \vxi(\alpha,\vphi)
        \right)
        \mid \mM_{:,2}, \mSigma)
        \\
        \propto
        &
        \exp\left(
            \sum_{n=1}^7 c_n\left(\alpha, \mM, \vr, \vphi\right)
        \right)
    \end{align*}
    with
    \begin{align*}
         c_1\left(\alpha, \mM, \vr, \vphi\right) &= -\frac{1}{2} \mM_{:,1} ^T \mSigma^{-1} \mM_{:,1} + \mM_{:,2} ^T \mSigma^{-1} \mM_{:,2},
        \\
        c_2\left(\alpha, \mM, \vr, \vphi\right) &= \left(
        \vr \odot \cos\left(
            \vxi(\alpha,\vphi)
        \right)
        \right) ^T \mSigma^{-1} \mM_{:,1} ,
        \\
        c_3\left(\alpha, \mM, \vr, \vphi\right)& = \left(
        \vr \odot \sin\left(
            \vxi(\alpha,\vphi)
        \right)
        \right) ^T \mSigma^{-1} \mM_{:,2},
        \\
        c_4\left(\alpha, \mM, \vr, \vphi\right) &= -\frac{1}{2} \sum_{n=1}^N \sum_{m=1}^N \mSigma^{-1}_{n,m} r_n r_m \cos\left(
            \vxi(\alpha,\vphi)
        \right)_n
        \cos\left(
            \vxi(\alpha,\vphi)
        \right)_m,
        \\
        c_5\left(\alpha, \mM, \vr, \vphi\right) &= -\frac{1}{2}  \sum_{n=1}^N \sum_{m=1}^N \mSigma^{-1}_{n,m} r_n r_m \sin\left(
            \vxi(\alpha,\vphi)
        \right)_n
        \sin\left(
            \vxi(\alpha,\vphi)
        \right)_m.
    \end{align*}
    Note that $c_4$ and $c5$ correspond to
    $-\frac{1}{2}\cos\left(
            \vxi(\alpha,\vphi)
        \right)^T \mSigma^{-1} \cos\left(
            \vxi(\alpha,\vphi)
        \right)$
    and
    $-\frac{1}{2}\sin\left(
            \vxi(\alpha,\vphi)
        \right)^T \mSigma^{-1} \sin\left(
            \vxi(\alpha,\vphi)
        \right)$, respectively.

    $c_1$ is constant in $\alpha$ and can thus be moved outside the integral.
    
    $c_2$ and $c_3$ are not constant in $\alpha$ and must therefore remain inside the integral.
    
    $c_4 + c_5$ can also be shown to be constant w.r.t.\ both $\mM$ and $\alpha$.
    By the trigonometric identity $\cos(a) \cos(b) + \sin(a) \sin(b) = \cos(a-b)$, we have
    \begin{align*}
        c_4\left(\alpha, \mM, \vr, \vphi\right)
        + c_5\left(\alpha, \mM, \vr, \vphi\right)
        =
        - \frac{1}{2} \sum_{n=1}^N \sum_{m=1}^N \mSigma^{-1}_{n,m} r_n r_m \cos\left(
            \evxi(\alpha,\vphi)_n - \evxi(\alpha,\vphi)_m
            \right).
    \end{align*}
    Recall that $\vxi(\alpha, \vphi) =
        \vphi + \ones_N \alpha$, i.e. ``$+\alpha$'' appears in every row.  Subtraction thus eliminates $\alpha$ for all combinations of $n$ and $m$.
            
    Based on these observations, we may conclude that
    \begin{align}
        &\int\limits_{[0,2\pi]} \mathcal{N}
        \left(\vr \odot \cos\left(
            \vxi(\alpha,\vphi)
        \right) \mid \mM_{:,1}, \mSigma \right)
        \mathcal{N}\left(\vr \odot \sin\left(
            \vxi(\alpha,\vphi)
        \right) \mid \mM_{:,2}, \mSigma \right) \ d \alpha
        \\\label{eq:bessel_integral_1}
        \propto & 
        \exp\left(c_1\left(\alpha, \mM, \vr, \vphi\right)\right)
        \int\limits_{[0,2\pi]}
        \exp\left(c_2\left(\alpha, \mM, \vr, \vphi\right) + c_3\left(\alpha, \mM, \vr, \vphi\right)\right)
        \ d \alpha.
    \end{align}
    Next, we use the trigonometric identites $\cos(a+b) = \cos(a) \cos(b) - \sin(a) \sin(b)$ and $\sin(a+b) = \sin(a) \cos(b) + \cos(a) \sin(b)$ to move $\alpha$ outside the inner products within $c_2$ and $c_3$:
    \begin{align*}
        &c_2\left(\alpha, \mM, \vr, \vphi\right)\\
        =& \left(
        \vr \odot \cos\left(
            \vxi(\alpha,\vphi)
        \right)
        \right) ^T \mSigma^{-1} \mM_{:,1}\\
        =&
        \left(
        \vr \odot \cos\left(
            \ones_{N} \alpha
            +
            \vphi
        \right)
        \right) ^T \mSigma^{-1} \mM_{:,1}\\
        =&
        \left(
        \vr \odot
        \cos\left(
        \ones_{N} \alpha\right)
        \odot
        \cos\left(
            \vphi
        \right)
        \right) ^T \mSigma^{-1} \mM_{:,1}
        - 
        \left(
        \vr \odot
        \sin\left(
        \ones_{N} \alpha\right)
        \odot
        \sin\left(
            \vphi
        \right)
        \right) ^T \mSigma^{-1} \mM_{:,1}
        \\
        = & 
        \cos(\alpha)
        \left(
        \vr \odot
        \cos\left(
            \vphi
        \right)
        \right) ^T \mSigma^{-1} \mM_{:,1}
        - 
        \sin(\alpha)
        \left(
        \vr \odot
        \sin\left(
            \vphi
        \right)
        \right) ^T \mSigma^{-1} \mM_{:,1} \\
        = & 
        \cos(\alpha)
        \lambda\left(\vr, \vphi\right)_{:,1}^T
        \mSigma^{-1} \mM_{:,1}
        -
        \sin(\alpha)
        \lambda\left(\vr, \vphi\right)_{:,2}^T
        \mSigma^{-1} \mM_{:,1}
    \end{align*}
    and
    \begin{align*}
        &c_3\left(\alpha, \mM, \vr, \vphi\right)\\
        =& \left(
        \vr \odot \sin\left(
            \vxi(\alpha,\vphi)
        \right)
        \right) ^T \mSigma^{-1} \mM_{:,2}\\
        =&
        \left(
        \vr \odot \sin\left(
            \ones_N \alpha + \vphi
        \right)
        \right) ^T \mSigma^{-1} \mM_{:,2}\\
        = & 
        \sin(\alpha)
        \left(
        \vr \odot
        \cos\left(
            \vphi
        \right)
        \right) ^T \mSigma^{-1} \mM_{:,2}
        +
        \cos(\alpha)
        \left(
        \vr \odot
        \sin\left(
            \vphi
        \right)
        \right) ^T \mSigma^{-1} \mM_{:,2} \\
        = & 
        \sin(\alpha)
        \lambda\left(\vr, \vphi\right)_{:,1}^T
        \mSigma^{-1} \mM_{:,2}
        +
        \cos(\alpha)
        \lambda\left(\vr, \vphi\right)_{:,2}^T
        \mSigma^{-1} \mM_{:,2}.
    \end{align*}
    Stacking the $\mSigma^{-1} \mM$ terms, we can express $c_2+c_3$ as follows:
    \begin{align*}
        &c_2\left(\alpha, \mM, \vr, \vphi\right) + c_3\left(\alpha, \mM, \vr, \vphi\right)
         \\
        = & cos(\alpha) 
        \begin{bmatrix}
            \mSigma^{-1} \mM_{:,1}\\
            \mSigma^{-1} \mM_{:,2}
        \end{bmatrix}^T
        \begin{bmatrix}
            \lambda\left(\vr, \vphi\right)_{:,1} \\
            \lambda\left(\vr, \vphi\right)_{:,2}
        \end{bmatrix}
        + cos(\alpha) 
        \begin{bmatrix}
            \mSigma^{-1} \mM_{:,2}\\
            -\mSigma^{-1} \mM_{:,1}
        \end{bmatrix}^T
        \begin{bmatrix}
            \lambda\left(\vr, \vphi\right)_{:,1} \\
            \lambda\left(\vr, \vphi\right)_{:,2}
        \end{bmatrix} \\
        \vcentcolon= & \cos(\alpha) \eta_1 \sin(\alpha) \eta_2.
    \end{align*}
    We can now substitute our results into ~\cref{eq:bessel_integral_1} and simplify the integral using the fact that
    $\cos(\alpha) \eta_1 + \sin(\alpha) \eta_2 =
    \cos(\alpha + \omega) \sqrt{\eta_1^2 + \eta_2^2)}
    $ \todo{cite}
    for some $\omega \in [0,1]$.
    \begin{align*}
    &\exp\left(c_1\left(\alpha, \mM, \vr, \vphi\right)\right)
        \int\limits_{[0,2\pi]}
        \exp\left(c_2\left(\alpha, \mM, \vr, \vphi\right) + c_3\left(\alpha, \mM, \vr, \vphi\right)\right)
        \ d \
    \\
    = &
    \exp\left(c_1\left(\alpha, \mM, \vr, \vphi\right)\right)
        \int\limits_{[0,2\pi]}
        \exp\left( \cos(\alpha) \eta_1 + \sin(\alpha) \eta_2 \right)
        \ d \alpha
    \\
    = &
    \exp\left(c_1\left(\alpha, \mM, \vr, \vphi\right)\right)
        \int\limits_{[0,2\pi]}
        \exp\left( \cos(\alpha + \omega) \sqrt{\eta_1^2 + \eta_2^2)} \right)
        \ d \alpha
    \\
    = &
    \exp\left(c_1\left(\alpha, \mM, \vr, \vphi\right)\right)
        \int\limits_{[0,2\pi]}
        \exp\left( \cos(\alpha) \sqrt{\eta_1^2 + \eta_2^2)} \right)
        \ d \alpha
    \\
    = &
    \exp\left(c_1\left(\alpha, \mM, \vr, \vphi\right)\right)
        \frac{\pi}{2} \mathcal{I}_0\left( \sqrt{\eta_1^2 + \eta_2^2)} \right),
    \end{align*}
    where the second to last equality is due to the fact that we integrate over an entire period of $\cos$ and the last equality uses the integral representation of the modified Bessel function of the first kind with order $0$:
    \begin{align*}
        \mathcal{I}_0(z) = \frac{1}{\pi} 
        =
        \int\limits_{[0,\pi]}
        \exp\left( \cos(\alpha) z  \right)
        \ d \alpha.
    \end{align*}
    Restating $\sqrt{\eta_1^2 + \eta_2^2)}$ as
    \begin{align*}
        \left\lvert\left\lvert
        \begin{bmatrix}
            \mSigma^{-1} \mM_{:,1}  & \mSigma^{-1} \mM_{:,2} \\
            \mSigma^{-1} \mM_{:,2} & -\mSigma^{-1} \mM_{:,1} 
        \end{bmatrix}^T
        \begin{bmatrix}
            \lambda\left(\vr, \vphi\right)_{:,1} \\
            \lambda\left(\vr, \vphi\right)_{:,2}
        \end{bmatrix}
        \right\rvert\right\rvert_2
    \end{align*}
    concludes our proof.
\end{proof}

\begin{proof}
    Applying~\cref{theorem:canonical_cert} with~\cref{lemma:canonical_representation_rotation_2d} shows that  the l.h.s.\ problem is equivalent to
    \begin{align*}
        \min_{h : \sR^{N \times D} \rightarrow \sY}   \Pr_{\mZ \sim \mu_{\mX'}} \left[h(\mK\mZ) = y^*\right]
    \text{ s.t. } \Pr_{\mZ \sim \mu_{\mX}} \left[h(\mK \mZ) = y^*\right] \geq p_{\mX, y^*}.
    \end{align*}
    
    Like in our previous proof, we notice that the above optimization problem does not depend on the specific class predicted by $h$, but only on whether it is $y^*$ or $y$. We thus formulate the equivalent problem 
    \begin{align}\label{eq:proof_rotation_2d_1}
        \min_{h : \sR^{N \times D} \rightarrow \{0,1\}}   \mathbb{E}_{\mZ \sim \mu_{\mX'}} \left[h(\gamma(\mZ))\right]
    \text{ s.t. } \mathbb{E}_{\mZ \sim \mu_{\mX}} \left[h(\gamma(\mZ))\right] \geq p_{\mX, y^*},
    \end{align}
    where $h(\mZ) = 1$ indicates that $\mZ$ is classified as $y^*$.
    
    Following the procedure outlined in~\cref{section:certification_methodology}, we now apply appropriately chosen substitutions to reduce the two expectation terms to expectations over a lower-dimensional distribution. We then apply the Neyman-Pearson lemma.

    We begin by going from cartesian to polar coordinates:
    As defined in the previous section, let
    $\lambda : \sR^N \times \sR^N \rightarrow \sR^{N \times 2}$ with
    $\lambda\left(\vr,\vtheta\right) =
    \begin{bmatrix}
        \vr \odot \cos(\vtheta) & \vr \odot \sin(\vtheta)
    \end{bmatrix}$
    be the function that maps from polar coordinates into cartesian coordiantes.
    \begin{align*}
        &\mathbb{E}_{\mZ \sim \mu_{\mX}} \left[h(\gamma(\mZ))\right]
        \\
        =
        &
        \int_{\sR^{N \times D}} h(\gamma(\mZ)) \mu_\mX(\mZ) \ d\mZ
        \\
        =
        &
        \int_{\sR^{N}}
        \left(\prod_{n=1}^N \evr_n\right)
        \int_{[0,2 \pi]^N} h(\gamma(\lambda(\vr,\vtheta))) \mu_\mX\left(\lambda(\vr, \vtheta)\right)) \ d \vtheta \ d \vr
    \end{align*}
    The $r_n$ in the last equality are due to the fact that $\lambda$ transforms $N$ rows from polar to Cartesian coordinates, with each transformation having a Jacobian $r$.
    Now, we would like to actually apply our canonical representation $\gamma$. Recall from~\cref{lemma:canonical_representation_rotation_2d} that $\lambda$ requires a case distinction to find the first non-zero row of $\lambda(\vr,\vtheta)$.
    However, due to the term $\prod_{n=1}^N \evr_n$, the entire integrand becomes zero whenever any row of $\lambda(\vr,\vtheta)$ is zero.
    We can therefore always assume that we are in the case with $\evr_1 > 0$, i.e.~\ rotate by $\evtheta_1$, without influencing the value of the integral.
    Thus
    \begin{align*}
        &\mathbb{E}_{\mZ \sim \mu_{\mX}} \left[h(\gamma(\mZ))\right]
        \\
        =
        &
        \int_{\sR^{N}}
        \left(\prod_{n=1}^N \evr_n\right)
        \int_{[0,2 \pi]^N} h\left(\lambda(\vr,\vtheta - \ones_N \evtheta_1)\right) \mu_\mX\left(\lambda(\vr, \vtheta)\right)) \ d \vtheta \ d \vr
    \end{align*}
    Next, we apply a similar substitution to the one used in our translation certificate:
    Let $\vpsi = \mA \vtheta$ with 
    $\mA =
    \begin{bmatrix}
        1 & \zeros_{N-1}^T\\
        -\ones_{N-1} & \eye_{N-1}
    \end{bmatrix}
    $
    and
    $\mA^{-1} = \begin{bmatrix}
        1 & \zeros_{N-1} \\
        \ones_{N-1} & \eye_N
    \end{bmatrix}$.
    Note that $\mA^{-1} \left(\vpsi - \ones_N \evpsi_1\right) = \begin{bmatrix}
        0 \\ \vpsi_{2:}
    \end{bmatrix}$
    ,
    where $\vpsi_{2:}$ is $\vpsi$ after removing the first entry.
    Further note that $\mathrm{det}\left(\mA^{-1}\right) = 1$ and that we have to adjust the integration boundaries, because we are now integrating over angle differences.
    \begin{align*}
        =
        &
        \int\limits_{\sR^{N}}
        \left(\prod_{n=1}^N \evr_n\right)
        \int\limits_{[0,2\pi]}
        \int\limits_{[-\evpsi_1,2 \pi-\evpsi_1]^{N-1}} h\left(\lambda\left(\vr,
            \begin{bmatrix}
            0 \\ \vpsi_{2:}
            \end{bmatrix}
        \right)\right) \mu_\mX\left(\lambda(\vr, \mA^{-1}\vpsi)\right)) \ d \vpsi_{2:} d \evpsi_1 \ d \vr.
    \end{align*}
    Note that $\lambda$ is $2\pi$-periodic w.r.t.\ its second argument
    and
    $\mA^{-1} \vpsi =
    \begin{bmatrix}
        \evpsi_1\\
        \vpsi_{2:} + \ones_{N-1} \evpsi_1
    \end{bmatrix}
    $
    , meaning that for any fixed $\vpsi_1$ integration over $[-\evpsi_1,2 \pi-\evpsi_1]^{N-1}$ is equivalent to integration over $[0, 2\pi]$. Further note that the term involving $h$ does not depend on $\vpsi$, meaning it can be moved out.
    \begin{align*}
        =
        &
        \int\limits_{\sR^{N}}
        \left(\prod_{n=1}^N \evr_n\right)
        \int\limits_{[0,2\pi]}
        \int\limits_{[0,2\pi]^{N-1}} h\left(\lambda\left(\vr,
            \begin{bmatrix}
            0 \\ \vpsi_{2:}
            \end{bmatrix}
        \right)\right) \mu_\mX\left(\lambda(\vr, \mA^{-1}\vpsi)\right)) \ d \vpsi_{2:} d \evpsi_1 \ d \vr
    \\
        =
        &
        \int\limits_{\sR^{N}}
        \int\limits_{[0,2\pi]^{N-1}}
        h\left(\lambda\left(\vr,
            \begin{bmatrix}
            0 \\ \vpsi_{2:}
            \end{bmatrix}
        \right)\right)
        \left(\prod_{n=1}^N \evr_n\right)
        \int\limits_{[0,2\pi]}
         \mu_\mX\left(\lambda(\vr, \mA^{-1}\vpsi)\right)) \ d \evpsi_1 d \vpsi_{2:}  \ d \vr
    \end{align*}
    This demonstrates that 
    $\mathbb{E}_{\mZ \sim \mu_{\mX}} \left[h(\gamma(\mZ))\right] = \mathbb{E}_{\vr, \vpsi_{2:} \sim \nu_{\mX}} \left[
    h\left(\lambda\left(\vr,
            \begin{bmatrix}
            0 \\ \vpsi_{2:}
            \end{bmatrix}
        \right)\right)
    \right]$
    with $\nu_\mX$ being a distribution over $\sR^N \times [0,2\pi]^{N-1}$ with density function
    \begin{align}
        \nu_\mX(\vr, \vpsi_{2:}) =
        &\left(\prod_{n=1}^N \evr_n\right)
        \int\limits_{[0,2\pi]}
         \mu_\mX\left(\lambda(\vr, \mA^{-1}\vpsi)\right)) \ d \evpsi_1
         \\ &
         \left(\prod_{n=1}^N \evr_n\right)
        \int\limits_{[0,2\pi]}
         \mu_\mX\left(\lambda\left(\vr, \begin{bmatrix}
            0 \\ \vpsi_{2:}
            \end{bmatrix}
            + \ones_N \evpsi_1
            \right)\right) \ d \evpsi_1
    \end{align}
    Substituting into~\cref{eq:proof_rotation_2d_2} and replacing $\vpsi_{2:}$ with $\vomega \in [0,2\pi]^{N-1}$ to clarify that we are sampling a new vector instead of indexing an existing one leaves us with the optimization problem.
    \begin{align}\label{eq:proof_rotation_2d_2}
    \begin{split}
        \min_{h : \sR^{N \times D} \rightarrow \{0,1\}}   
        &\mathbb{E}_{\vr, \vomega \sim \nu_{\mX'}} \left[
    h\left(\lambda\left(\vr,
            \begin{bmatrix}
            0 \\ \vomega
            \end{bmatrix}
        \right)\right)
    \right]\\
    \text{ s.t. } 
    &\mathbb{E}_{\vr, \vomega \sim \nu_{\mX}} \left[
    h\left(\lambda\left(\vr,
            \begin{bmatrix}
            0 \\ \vomega
            \end{bmatrix}
        \right)\right)
    \right]
    \geq p_{\mX, y^*}.
    \end{split}
    \end{align}
    Note that $\lambda$ is an injective function from $\sR^N \times [0,2\pi]^{N}$ into $\sR^{N \times D}$, meaning that each pair $(\vr, \omega)$ in the support of $\nu_{\mX}$ and $\nu_{\mX'}$ corresponds to a distinct function value $h(\mZ)$.
    We may thus equivalently find the worst-case classifier in $\sR^{N} \times [0,2\pi]^{N-1}$:
    \begin{align}
        \min_{h : \sR^{N} \times [0,2\pi]^{N-1} \rightarrow \{0,1\}}   \mathbb{E}_{\vr, \vomega \sim \mu_{\mX'}} \left[h(\vr, \vomega)\right]
    \text{ s.t. } \mathbb{E}_{\vr, \vomega \sim \mu_{\mX}}  \left[h(\vr, \vomega)\right] \geq p_{\mX, y^*}.
    \end{align}
    Applying the Neyman Pearson lemma to the above problem shows that its optimal value is
    \begin{align}\label{eq:neyman_pearson_rotation}
        & \mathbb{E}_{\vr, \vomega \sim \mu_{\mX'}} \left[h^*(\vr,\vomega)\right] \\
        \text{with } & h^*(\vr,\vomega) = \indicator\left[\frac{\nu_{\mX'}(\vr,\vomega)}{\nu_{\mX}(\vr,\vomega)} \leq t\right] \text{ and } t \in \sR \text{ s.t. }
        \mathbb{E}_{\vr, \vomega \sim \mu_{\mX}} \left[h^*(\vr,\vomega)\right] = p_{\mX, y^*}.
    \end{align}
    To conclude our proof, we transform the expectations over the lower-dimensional space of representatives in~\cref{eq:neyman_pearson_rotation} back to our Cartesian space $\sR^{N \times D}$.
    Before doing so, we take a minor precaution to make the integration bounds easier to work with.
    We define the function $\hat{h} : \sR^{N} \times \sR^{N-1} \rightarrow \{0,1\}$ with
    $\hat{h}(\vr,\vomega) = h^*(\vr,(\chi(\omega))$, where $\chi(\omega) = \omega + 2 k \pi$ s.t.\ $\omega + 2 k \in [0,2\pi]$.
    Clearly $\mathbb{E}_{\vr, \vomega \sim \mu_{\mX'}} \left[\hat{h}(\vr,\vomega)\right]$ = $\mathbb{E}_{\vr, \vomega \sim \mu_{\mX'}} \left[h^*(\vr,\vomega)\right]$.
    Therefore
    \begin{align*}
        & \mathbb{E}_{\vr, \vomega \sim \mu_{\mX}} \left[h^*(\vr,\vomega)\right]
        \\
        =
        &
        \int\limits_{\sR^{N} \times [0,2\pi]^{N-1}}
        \hat{h}(\vr,\vomega)
        \nu_{\mX}(\vr,\vomega) \ d \vomega \ d \vr
        \\
        =
        &
        \int\limits_{\sR^{N} \times [0,2\pi]^{N-1}}
        \hat{h}(\vr,\vomega)
        \left(\prod_{n=1}^N \evr_n\right)
        \int\limits_{[0,2\pi]}
         \mu_\mX\left(\lambda\left(\vr, \begin{bmatrix}
            0 \\ \vomega
            \end{bmatrix}
            + \ones_N \beta
            \right)\right) \ d \beta \ d \vomega \ d \vr
        \\
        =
        &
        \int\limits_{\sR^{N} \times [0,2\pi]^{N}}
        \hat{h}(\vr,\vomega)
        \left(\prod_{n=1}^N \evr_n\right)
         \mu_\mX\left(\lambda\left(\vr, \begin{bmatrix}
            0 \\ \vomega
            \end{bmatrix}
            + \ones_N \beta
            \right)\right) \  \ d \vomega d \beta \ d \vr
        \\
    \end{align*}
    We now use the substitution $\vtheta = \mA^{-1} \begin{bmatrix}
    \beta \\
    \vomega
    \end{bmatrix}$
    with 
    $\mA^{-1} = \begin{bmatrix}
        1 & \zeros_{N-1} \\
        \ones_{N-1} & \eye_N
    \end{bmatrix}$
    to transform back into standard polar coordinates and use the fact that all functions are $2\pi$-periodic for any fixed $\evtheta_1$ to simplify the integration bounds.
    \begin{align*}
        & 
        \int\limits_{\sR^{N} \times [0,2\pi] \times [\evtheta_1,2\pi+\evtheta_1]^{N}}
        \hat{h}(\vr,\vomega - \ones_{N-1} \evtheta_1)
        \left(\prod_{n=1}^N \evr_n\right)
         \mu_\mX\left(\lambda\left(\vr, \vtheta
            \right)\right) \ d \theta_{2:} \ d \evtheta_1 \ d \vr
        \\
        = & \int\limits_{\sR^{N} \times [0,2\pi]^N }
        \hat{h}(\vr,\vomega - \ones_{N-1} \evtheta_1)
        \left(\prod_{n=1}^N \evr_n\right)
         \mu_\mX\left(\lambda\left(\vr, \vtheta
            \right)\right) \ d \vtheta \ d \vr.
        \\
    \end{align*}
    
    Finally: Use lemma. Transform back into cartesian coordinates
\end{proof}
